# Supplementary material for: Excitons under large pseudomagnetic fields
Source: arXiv:2412.16596 source file (2024-12-21)

**a**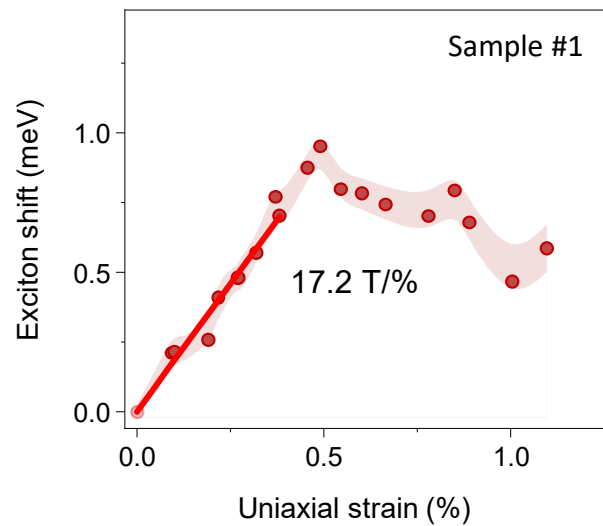**b**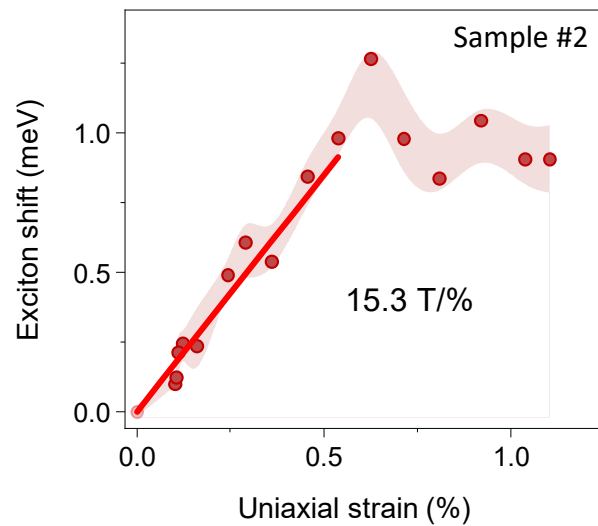**c**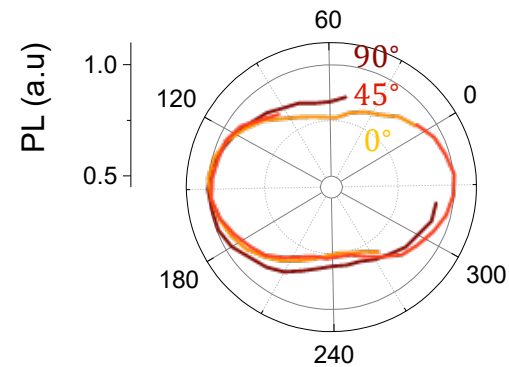**d**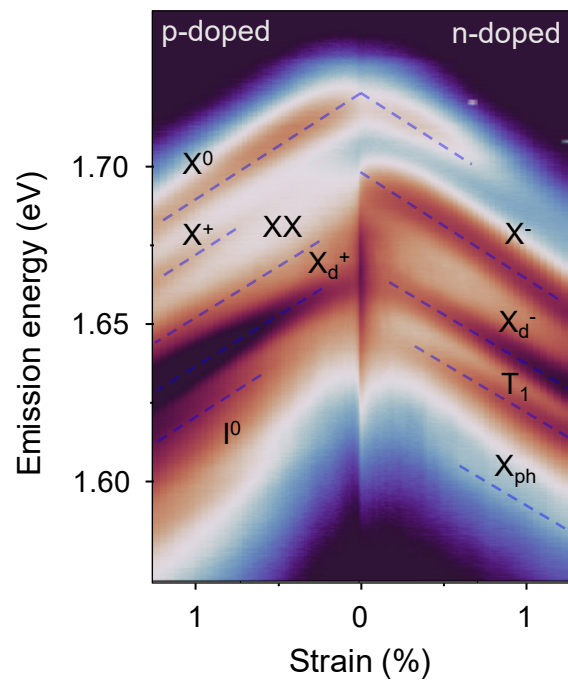**e**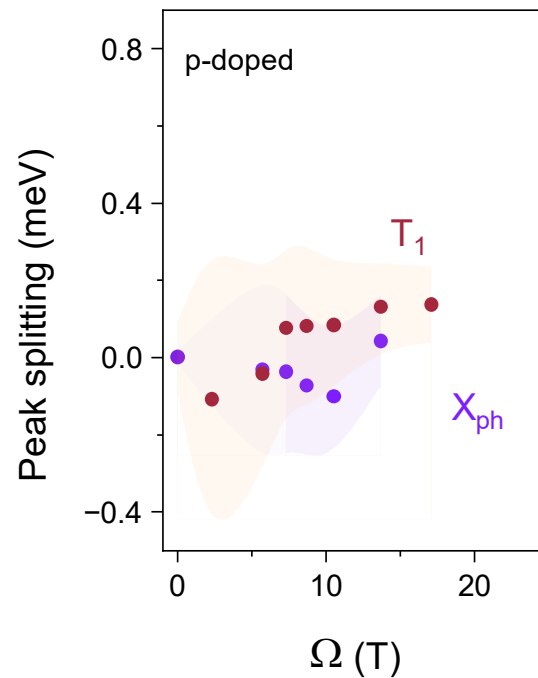**f**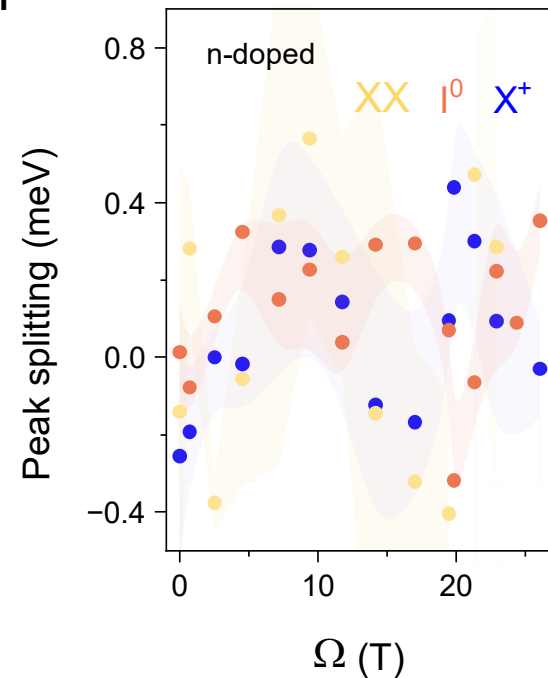

Supplement: Supplementary file 2 [file extened_WSe2_analysis.pdf]
